# Supplementary material for: The Effect of Natural Distribution Shift on Question Answering Models
Source: arXiv:2004.14444 source file (2020-04-29)
Supplement: Supplementary file 1 [file appendix_em_table.tex]

\rowcolors{2}{gray!15}{white}
\begin{tabular}{llccccc}
    \toprule
    \multicolumn{7}{c}{\textbf{EM Score}} \\
    \midrule
        Name & Rank & SQuAD v1.1 & New-Wiki & NYT & Reddit  & Amazon  \\
    \midrule
	Human-0 & - & 89.1  \textcolor{gray!70}{[87.1, 91.0]} & 82.6  \textcolor{gray!70}{[80.0, 85.0]} & 86.0  \textcolor{gray!70}{[83.6, 88.1]} & 80.1  \textcolor{gray!70}{[77.2, 82.7]} & 79.9  \textcolor{gray!70}{[77.1, 82.4]} \\
	Human-1 & - & 88.7  \textcolor{gray!70}{[86.6, 90.6]} & 83.2  \textcolor{gray!70}{[80.6, 85.6]} & 88.5  \textcolor{gray!70}{[86.3, 90.5]} & 80.7  \textcolor{gray!70}{[77.8, 83.3]} & 81.1  \textcolor{gray!70}{[78.4, 83.6]} \\
	Human-2 & - & 90.5  \textcolor{gray!70}{[88.5, 92.2]} & 85.4  \textcolor{gray!70}{[82.9, 87.6]} & 85.8  \textcolor{gray!70}{[83.4, 87.9]} & 81.0  \textcolor{gray!70}{[78.2, 83.6]} & 79.3  \textcolor{gray!70}{[76.5, 82.0]} \\
	XLNET-123  & 2 & 89.6 & 84.0  \textcolor{gray!70}{[83.1, 84.8]} & 86.3  \textcolor{gray!70}{[85.6, 87.0]} & 74.2  \textcolor{gray!70}{[73.2, 75.1]} & 73.8  \textcolor{gray!70}{[72.8, 74.7]} \\
	Tuned BERT-1seq Large C & 5 & 87.5 & 82.3  \textcolor{gray!70}{[81.3, 83.2]} & 83.7  \textcolor{gray!70}{[83.0, 84.5]} & 71.0  \textcolor{gray!70}{[70.0, 72.0]} & 71.3  \textcolor{gray!70}{[70.2, 72.2]} \\
	BERT-Large Baseline  & 7 & 86.6 & 82.0  \textcolor{gray!70}{[81.1, 82.9]} & 83.4  \textcolor{gray!70}{[82.6, 84.1]} & 69.6  \textcolor{gray!70}{[68.6, 70.6]} & 68.5  \textcolor{gray!70}{[67.4, 69.5]} \\
	DPN  & 10 & 85.0 & 80.2  \textcolor{gray!70}{[79.2, 81.2]} & 80.5  \textcolor{gray!70}{[79.6, 81.3]} & 67.1  \textcolor{gray!70}{[66.1, 68.2]} & 65.3  \textcolor{gray!70}{[64.3, 66.4]} \\
	Common-sense Governed B & 10 & 83.9 & 78.6  \textcolor{gray!70}{[77.6, 79.6]} & 79.5  \textcolor{gray!70}{[78.6, 80.3]} & 68.1  \textcolor{gray!70}{[67.1, 69.1]} & 67.2  \textcolor{gray!70}{[66.2, 68.2]} \\
	BISAN  & 10 & 85.3 & 79.9  \textcolor{gray!70}{[78.9, 80.8]} & 80.6  \textcolor{gray!70}{[79.8, 81.4]} & 68.4  \textcolor{gray!70}{[67.4, 69.4]} & 66.9  \textcolor{gray!70}{[65.8, 67.9]} \\
	BERT+Sparse-Transformer & 10 & 85.1 & 80.2  \textcolor{gray!70}{[79.2, 81.1]} & 80.3  \textcolor{gray!70}{[79.4, 81.1]} & 69.1  \textcolor{gray!70}{[68.0, 70.1]} & 67.6  \textcolor{gray!70}{[66.6, 68.6]} \\
	Original BERT Large Cas & 11 & 84.3 & 80.5  \textcolor{gray!70}{[79.5, 81.5]} & 80.4  \textcolor{gray!70}{[79.6, 81.2]} & 68.3  \textcolor{gray!70}{[67.3, 69.3]} & 66.2  \textcolor{gray!70}{[65.2, 67.2]} \\
	InfoWord-Base  & 11 & 84.7 & 80.5  \textcolor{gray!70}{[79.6, 81.5]} & 80.8  \textcolor{gray!70}{[80.0, 81.6]} & 66.8  \textcolor{gray!70}{[65.7, 67.8]} & 65.0  \textcolor{gray!70}{[63.9, 66.0]} \\
	MARS  & 13 & 83.2 & 76.3  \textcolor{gray!70}{[75.2, 77.3]} & 75.2  \textcolor{gray!70}{[74.3, 76.1]} & 59.9  \textcolor{gray!70}{[58.8, 60.9]} & 54.9  \textcolor{gray!70}{[53.8, 56.0]} \\
	MMIPN  & 15 & 81.6 & 77.4  \textcolor{gray!70}{[76.4, 78.4]} & 77.0  \textcolor{gray!70}{[76.1, 77.9]} & 63.6  \textcolor{gray!70}{[62.6, 64.7]} & 62.2  \textcolor{gray!70}{[61.1, 63.3]} \\
	{EAZI} (ensemble) & 18 & 80.4 & 75.5  \textcolor{gray!70}{[74.4, 76.5]} & 76.0  \textcolor{gray!70}{[75.1, 76.9]} & 62.0  \textcolor{gray!70}{[60.9, 63.0]} & 58.6  \textcolor{gray!70}{[57.5, 59.6]} \\
	BiDAF + Self Attention  & 25 & 78.6 & 73.4  \textcolor{gray!70}{[72.4, 74.5]} & 74.5  \textcolor{gray!70}{[73.5, 75.4]} & 59.7  \textcolor{gray!70}{[58.6, 60.8]} & 56.3  \textcolor{gray!70}{[55.2, 57.4]} \\
	MEMEN  & 27 & 78.2 & 73.7  \textcolor{gray!70}{[72.6, 74.7]} & 71.0  \textcolor{gray!70}{[70.0, 71.9]} & 60.0  \textcolor{gray!70}{[58.9, 61.1]} & 56.4  \textcolor{gray!70}{[55.3, 57.5]} \\
	EAZI  & 29 & 78.0 & 73.8  \textcolor{gray!70}{[72.8, 74.9]} & 73.1  \textcolor{gray!70}{[72.1, 74.0]} & 58.3  \textcolor{gray!70}{[57.2, 59.4]} & 55.0  \textcolor{gray!70}{[53.9, 56.1]} \\
	DNET  & 29 & 77.6 & 72.8  \textcolor{gray!70}{[71.7, 73.9]} & 73.2  \textcolor{gray!70}{[72.3, 74.1]} & 58.9  \textcolor{gray!70}{[57.8, 60.0]} & 56.1  \textcolor{gray!70}{[55.0, 57.2]} \\
	{gqa}  & 31 & 77.1 & 73.3  \textcolor{gray!70}{[72.2, 74.4]} & 70.3  \textcolor{gray!70}{[69.3, 71.2]} & 54.3  \textcolor{gray!70}{[53.2, 55.4]} & 51.8  \textcolor{gray!70}{[50.7, 52.9]} \\
	Jenga  & 38 & 74.4 & 68.6  \textcolor{gray!70}{[67.5, 69.7]} & 67.1  \textcolor{gray!70}{[66.1, 68.1]} & 52.3  \textcolor{gray!70}{[51.2, 53.4]} & 49.4  \textcolor{gray!70}{[48.3, 50.5]} \\
	AVIQA  & 44 & 72.5 & 69.9  \textcolor{gray!70}{[68.8, 71.0]} & 68.8  \textcolor{gray!70}{[67.8, 69.7]} & 54.6  \textcolor{gray!70}{[53.5, 55.7]} & 51.4  \textcolor{gray!70}{[50.3, 52.5]} \\
	M-NET  & 47 & 71.0 & 67.2  \textcolor{gray!70}{[66.0, 68.3]} & 65.5  \textcolor{gray!70}{[64.5, 66.5]} & 46.5  \textcolor{gray!70}{[45.4, 47.6]} & 42.9  \textcolor{gray!70}{[41.8, 44.0]} \\
	SimpleBaseline  & 49 & 69.6 & 65.7  \textcolor{gray!70}{[64.6, 66.9]} & 66.2  \textcolor{gray!70}{[65.2, 67.2]} & 48.7  \textcolor{gray!70}{[47.6, 49.8]} & 43.5  \textcolor{gray!70}{[42.4, 44.6]} \\
	AllenNLP BiDAF  & 53 & 68.0 & 64.8  \textcolor{gray!70}{[63.7, 66.0]} & 63.5  \textcolor{gray!70}{[62.5, 64.5]} & 44.1  \textcolor{gray!70}{[43.0, 45.2]} & 41.2  \textcolor{gray!70}{[40.1, 42.3]} \\
	RQA+IDR  & 61 & 61.1 & 53.6  \textcolor{gray!70}{[52.4, 54.9]} & 56.8  \textcolor{gray!70}{[55.8, 57.9]} & 46.2  \textcolor{gray!70}{[45.1, 47.3]} & 45.3  \textcolor{gray!70}{[44.2, 46.4]} \\
	UQA  & 63 & 53.7 & 47.8  \textcolor{gray!70}{[46.6, 49.0]} & 49.0  \textcolor{gray!70}{[47.9, 50.0]} & 34.9  \textcolor{gray!70}{[33.9, 36.0]} & 33.5  \textcolor{gray!70}{[32.5, 34.6]} \\
	UnsupervisedQA V1 & 65 & 44.2 & 39.9  \textcolor{gray!70}{[38.7, 41.0]} & 40.4  \textcolor{gray!70}{[39.3, 41.4]} & 35.5  \textcolor{gray!70}{[34.5, 36.6]} & 31.9  \textcolor{gray!70}{[30.9, 32.9]} \\
	\bottomrule
\end{tabular}
