# Supplementary material for: The Effect of Natural Distribution Shift on Question Answering Models
Source: arXiv:2004.14444 source file (2020-04-29)
Supplement: Supplementary file 2 [file appendix_f1_table.tex]

\rowcolors{2}{gray!15}{white}
\begin{tabular}{llccccc}
    \toprule
    \multicolumn{7}{c}{\textbf{F1 Score}} \\
    \midrule
        Name & Rank & SQuADv1.1 & New-Wiki & NYT & Reddit  & Amazon  \\
    \midrule
	Human-0 & - & 94.9  \textcolor{gray!70}{[93.8, 96.0]} & 92.5  \textcolor{gray!70}{[91.1, 93.8]} & 95.0  \textcolor{gray!70}{[93.9, 96.1]} & 92.4  \textcolor{gray!70}{[91.1, 93.7]} & 92.6  \textcolor{gray!70}{[91.3, 93.9]} \\
	Human-1 & - & 94.9  \textcolor{gray!70}{[93.8, 96.0]} & 92.4  \textcolor{gray!70}{[91.0, 93.8]} & 96.3  \textcolor{gray!70}{[95.4, 97.1]} & 92.6  \textcolor{gray!70}{[91.3, 93.9]} & 92.4  \textcolor{gray!70}{[91.1, 93.7]} \\
	Human-2 & - & 95.6  \textcolor{gray!70}{[94.5, 96.6]} & 92.3  \textcolor{gray!70}{[90.8, 93.8]} & 93.7  \textcolor{gray!70}{[92.4, 95.0]} & 91.7  \textcolor{gray!70}{[90.2, 93.2]} & 91.2  \textcolor{gray!70}{[89.6, 92.8]} \\
	XLNET-123  & 2 & 94.9 & 92.6  \textcolor{gray!70}{[92.1, 93.1]} & 93.2  \textcolor{gray!70}{[92.8, 93.6]} & 85.6  \textcolor{gray!70}{[85.0, 86.3]} & 87.1  \textcolor{gray!70}{[86.5, 87.7]} \\
	Tuned BERT-1seq Large C & 5 & 93.3 & 91.4  \textcolor{gray!70}{[90.9, 92.0]} & 91.2  \textcolor{gray!70}{[90.7, 91.7]} & 82.9  \textcolor{gray!70}{[82.1, 83.6]} & 84.3  \textcolor{gray!70}{[83.6, 84.9]} \\
	BERT-Large Baseline  & 7 & 92.7 & 91.3  \textcolor{gray!70}{[90.7, 91.8]} & 91.1  \textcolor{gray!70}{[90.6, 91.6]} & 82.3  \textcolor{gray!70}{[81.6, 83.0]} & 82.5  \textcolor{gray!70}{[81.8, 83.2]} \\
	DPN  & 10 & 92.0 & 90.4  \textcolor{gray!70}{[89.8, 91.0]} & 89.3  \textcolor{gray!70}{[88.8, 89.8]} & 81.1  \textcolor{gray!70}{[80.4, 81.8]} & 80.9  \textcolor{gray!70}{[80.2, 81.7]} \\
	Common-sense Governed B & 10 & 90.6 & 88.7  \textcolor{gray!70}{[88.1, 89.4]} & 87.8  \textcolor{gray!70}{[87.2, 88.4]} & 80.8  \textcolor{gray!70}{[80.0, 81.5]} & 80.1  \textcolor{gray!70}{[79.3, 80.8]} \\
	BISAN  & 10 & 91.8 & 89.9  \textcolor{gray!70}{[89.3, 90.5]} & 89.0  \textcolor{gray!70}{[88.5, 89.6]} & 81.4  \textcolor{gray!70}{[80.7, 82.1]} & 80.9  \textcolor{gray!70}{[80.2, 81.6]} \\
	BERT+Sparse-Transformer & 10 & 91.6 & 89.9  \textcolor{gray!70}{[89.3, 90.5]} & 89.0  \textcolor{gray!70}{[88.4, 89.6]} & 81.8  \textcolor{gray!70}{[81.1, 82.6]} & 81.4  \textcolor{gray!70}{[80.7, 82.2]} \\
	Original BERT Large Cas & 11 & 91.3 & 90.3  \textcolor{gray!70}{[89.7, 90.9]} & 89.0  \textcolor{gray!70}{[88.5, 89.6]} & 81.2  \textcolor{gray!70}{[80.5, 82.0]} & 80.7  \textcolor{gray!70}{[80.0, 81.4]} \\
	InfoWord-Base  & 11 & 91.4 & 90.0  \textcolor{gray!70}{[89.4, 90.6]} & 89.0  \textcolor{gray!70}{[88.5, 89.6]} & 79.7  \textcolor{gray!70}{[79.0, 80.5]} & 79.7  \textcolor{gray!70}{[79.0, 80.5]} \\
	MARS  & 13 & 89.5 & 86.4  \textcolor{gray!70}{[85.7, 87.1]} & 84.0  \textcolor{gray!70}{[83.3, 84.7]} & 73.9  \textcolor{gray!70}{[73.1, 74.8]} & 70.4  \textcolor{gray!70}{[69.5, 71.2]} \\
	MMIPN  & 15 & 88.9 & 87.8  \textcolor{gray!70}{[87.1, 88.4]} & 86.4  \textcolor{gray!70}{[85.8, 87.0]} & 77.3  \textcolor{gray!70}{[76.5, 78.1]} & 76.5  \textcolor{gray!70}{[75.7, 77.3]} \\
	{EAZI} (ensemble) & 18 & 86.9 & 85.6  \textcolor{gray!70}{[84.9, 86.3]} & 84.3  \textcolor{gray!70}{[83.7, 85.0]} & 74.6  \textcolor{gray!70}{[73.7, 75.4]} & 72.1  \textcolor{gray!70}{[71.2, 73.0]} \\
	BiDAF + Self Attention  & 25 & 85.9 & 84.2  \textcolor{gray!70}{[83.5, 85.0]} & 83.3  \textcolor{gray!70}{[82.6, 84.0]} & 72.9  \textcolor{gray!70}{[72.1, 73.8]} & 70.4  \textcolor{gray!70}{[69.5, 71.3]} \\
	MEMEN  & 27 & 85.3 & 84.1  \textcolor{gray!70}{[83.4, 84.9]} & 81.2  \textcolor{gray!70}{[80.5, 81.9]} & 72.9  \textcolor{gray!70}{[72.0, 73.8]} & 70.3  \textcolor{gray!70}{[69.4, 71.1]} \\
	EAZI  & 29 & 85.1 & 84.7  \textcolor{gray!70}{[83.9, 85.4]} & 82.4  \textcolor{gray!70}{[81.7, 83.1]} & 72.2  \textcolor{gray!70}{[71.3, 73.1]} & 69.5  \textcolor{gray!70}{[68.6, 70.4]} \\
	DNET  & 29 & 84.9 & 83.8  \textcolor{gray!70}{[83.1, 84.6]} & 82.1  \textcolor{gray!70}{[81.4, 82.9]} & 72.3  \textcolor{gray!70}{[71.4, 73.2]} & 70.2  \textcolor{gray!70}{[69.4, 71.1]} \\
	{gqa}  & 31 & 83.9 & 82.9  \textcolor{gray!70}{[82.1, 83.7]} & 78.7  \textcolor{gray!70}{[77.9, 79.5]} & 66.1  \textcolor{gray!70}{[65.2, 67.1]} & 64.1  \textcolor{gray!70}{[63.2, 65.1]} \\
	Jenga  & 38 & 82.8 & 80.6  \textcolor{gray!70}{[79.7, 81.4]} & 77.8  \textcolor{gray!70}{[77.0, 78.6]} & 67.7  \textcolor{gray!70}{[66.8, 68.6]} & 65.5  \textcolor{gray!70}{[64.6, 66.4]} \\
	AVIQA  & 44 & 80.5 & 80.7  \textcolor{gray!70}{[79.9, 81.6]} & 78.3  \textcolor{gray!70}{[77.5, 79.1]} & 68.0  \textcolor{gray!70}{[67.1, 68.9]} & 65.6  \textcolor{gray!70}{[64.7, 66.6]} \\
	M-NET  & 47 & 79.8 & 79.4  \textcolor{gray!70}{[78.5, 80.2]} & 76.2  \textcolor{gray!70}{[75.4, 77.0]} & 62.2  \textcolor{gray!70}{[61.3, 63.2]} & 59.5  \textcolor{gray!70}{[58.6, 60.5]} \\
	SimpleBaseline  & 49 & 78.2 & 78.0  \textcolor{gray!70}{[77.1, 78.9]} & 76.1  \textcolor{gray!70}{[75.3, 76.9]} & 63.3  \textcolor{gray!70}{[62.3, 64.2]} & 59.1  \textcolor{gray!70}{[58.2, 60.1]} \\
	AllenNLP BiDAF  & 53 & 77.3 & 77.0  \textcolor{gray!70}{[76.1, 77.9]} & 74.2  \textcolor{gray!70}{[73.4, 75.1]} & 60.0  \textcolor{gray!70}{[59.1, 60.9]} & 57.8  \textcolor{gray!70}{[56.8, 58.7]} \\
	RQA+IDR  & 61 & 71.4 & 67.0  \textcolor{gray!70}{[66.0, 68.0]} & 68.5  \textcolor{gray!70}{[67.6, 69.3]} & 59.3  \textcolor{gray!70}{[58.4, 60.3]} & 59.3  \textcolor{gray!70}{[58.4, 60.3]} \\
	UQA  & 63 & 64.0 & 61.5  \textcolor{gray!70}{[60.4, 62.5]} & 59.8  \textcolor{gray!70}{[58.9, 60.7]} & 46.9  \textcolor{gray!70}{[45.9, 47.9]} & 45.9  \textcolor{gray!70}{[44.9, 46.9]} \\
	UnsupervisedQA V1 & 65 & 54.7 & 53.5  \textcolor{gray!70}{[52.4, 54.6]} & 51.7  \textcolor{gray!70}{[50.8, 52.7]} & 48.5  \textcolor{gray!70}{[47.5, 49.5]} & 45.1  \textcolor{gray!70}{[44.2, 46.1]} \\
	\bottomrule
\end{tabular}
